# Supplementary material for: Incentivising Exploration and Recommendations for Contextual Bandits with Payments
Source: arXiv:2001.07853 source file (2020-01-22)
Supplement: Supplementary file 1 [file appendix.tex]

\newpage
\appendix

\section{Detailed Algorithms}\label{appd:detailed_algorithms}
We present here the pseudocodes of some of the algorithms which could not be accommodated in the main paper.\\

\textbf{Algorithm from Approach 1 ( Section~\ref{sec:algorithm:unrestricted})}:\\
\begin{algorithm}[H]
\SetKwFunction{CalcPayment}{CalcPayment}
\SetKwFunction{UpdateEstimate}{UpdateEstimate}
\SetKwFunction{InitialExploration}{InitialExploration}
\textbf{Input:} Arms: $\arms$, time horizon: $T$, contextual bandit algorithm: \textit{Alg}, and initial exploration parameter: $m$.\\
\InitialExploration{}\\
\For{ $t=m+1$ to $T$}{
Agent with context $\theta_t$ arrive at the Platform.\\
\textit{Principal calculates Payment:}\\
\quad\quad $\mathbf{p^t}$ = \CalcPayment{$\{\{\est^{t-1}_{i}\}, i \in [\arms]\,,\{\theta_s\}_{1}^{t}\}$, \textit{Alg}}\\
Agent choose arm $\pi_t = \arg\max_i (\est_i^t.\theta_t \, + p^t_{i})$.\\
\textit{Principal updates estimate $\mu_{\pi_t}$:}\\
\quad\quad \UpdateEstimate{} \\
}
\SetKwProg{myproc}{Procedure}{}{}
\myproc{\CalcPayment{}}{
\textit{Initialize:} $p^t_i = 0$, $i \in [\arms]$.\\  
$\pi_t^G$ = $\arg\max_i \est_i^t.\theta_t$.\\
$\pi_t^A$ = arm choice due to \textit{Alg} for current history.\\
\If{$\pi_t^G \neq \pi_t^A$ }{

$p^t_{\pi_t^A} = \max((\est_{\pi_t^G} - \est_{\pi_t^A}).\theta_t,0)$.\\
% $p^t_{j} = 0\, \forall j \neq \pi_t^G$.\\
}
\textbf{return} $\mathbf{p^t}$
}
\myproc{\UpdateEstimate{}}{ ( Same as that in \textit{Alg} e.g. $L_2$ loss minimization)
$\est_{\pi_t}^{t+1} = (\Theta(S_{\pi_t,t})^T\Theta(S_{\pi_t,t}))^{-1}\Theta(S_{\pi_t,t})^TY(S_{\pi_t,t})$.\\
}
\myproc{\InitialExploration{}}{
Platform makes $m$ observations using $\{\{\theta_t\}_{t=1}^m\}$ to get estimates $\{\{\est^m_{i}\}_{i \in \arms}\}$.\\
}
\caption{\PaymentProfile}\label{alg:Payment_Profile_Principal}
\end{algorithm}

\textbf{Algorithm from Approach 3 ( Section~\ref{sec:algorithm:unrestricted})}:\\
\begin{algorithm}[H]
\SetKwFunction{ConfidenceWidth}{ConfidenceWidth}
\SetKwFunction{UpdateEstimate}{UpdateEstimate}
\SetKwFunction{CalculatePayment}{CalculatePayment}
\SetKwFunction{InitialExploration}{InitialExploration}
\SetKwFunction{ChainedActions}{ChainedActions}
\textbf{Input:} Arms: $\arms$, time horizon: $T$, initial exploration parameter: $m$, ridge parameter: $\lambda$, and confidence parameter: $\delta$.\\
\InitialExploration{}\\
\For{ $t=m+1$ to $T$}{
Agent with context $\theta_t$ arrive at the Platform.\\
$\{\mathbf{p}^t_i\}_{i \in \arms}=$ \CalculatePayment{}.\\
Agent chooses arm $\arg \max \theta_t.(\est^t_i)+p^t_i$.\\
\UpdateEstimate{} \\
}
\SetKwProg{myproc}{Procedure}{}{}
\myproc{\CalculatePayment{}}{
\textit{Initialize:} $p^t_i = 0$, $i \in [\arms]$.\\ Agent's choice before payments: $i^t = \arg \max_{i\in\,[N]} \theta_t.\est^t_i$.\\
$\{w^t_i\}_{i \in \arms} =$ \ConfidenceWidth($\delta$). (see description in text)\\
$C^t_{i_t}=$ \ChainedActions($\{w^t_i\}_{i \in \arms}$). (see description in text)\\
$j =$ Uniformly random selection from $C^t_{i_t}$.\\
$p^t_j = \theta_t.(\est^t_{i_t} - \est^t_j)$.\\
\textbf{return} $\mathbf{p^t}$
}
\myproc{\UpdateEstimate{}}{
\textit{Updating history:}\\
\quad\quad $\Theta(S_{\pi_t,t+1}) = [\Theta(S_{\pi_t,t}) \vert \theta_t]$, and\\ \quad\quad $Y(S_{\pi_t,t+1}) = [Y(S_{\pi_t,t})\vert \est_{\pi_t}.\theta_t]$.\\
\textit{Updating Parameter:}\\
\quad\quad $\est_{\pi_t}^{t+1} = (\Theta(S_{\pi_t,t})^T\Theta(S_{\pi_t,t}) + \lambda I)^{-1}\Theta(S_{\pi_t,t})^TY(S_{\pi_t,t})$.\\
}
\caption{\UnrestrictedBudget}\label{alg:Unrestricted_Budget}
\end{algorithm}

\textbf{Algorithm from Approach 3 in the restricted budget setting ( Section~\ref{sec:algorithm:restricted})}:\\
\begin{algorithm}
\SetKwFunction{ConfidenceWidth}{ConfidenceWidth}
\SetKwFunction{UpdateEstimate}{UpdateEstimate}
\SetKwFunction{CalculatePayment}{CalculatePayment}
\SetKwFunction{InitialExploration}{InitialExploration}
\SetKwFunction{ChainedActions}{ChainedActions}
\textbf{Input:} Arms: $\arms$, time horizon: $T$, payment budget: $B$, initial exploration parameter: $m$, ridge parameter: $\lambda$, and confidence parameter: $\delta$.\\
\InitialExploration{}\\
\For{ $t=m+1$ to $T$}{
Agent with context $\theta_t$ arrive at the Platform.\\
$\{\mathbf{p}^t_i\}_{i \in \arms}=$ \CalculatePayment{}.\\
Agent chooses arm $\arg \max \theta_t.(\est^t_i)+p^t_i$.\\
\UpdateEstimate{} \\
}
\SetKwProg{myproc}{Procedure}{}{}
\myproc{\CalculatePayment{}}{
\textit{Initialize:} $p^t_i = 0$, $i \in [\arms]$.\\
\If{ $B$ > 0}{
Agent's choice before payments: $i^t = \arg \max_{i\in\,[N]} \theta_t.\est^t_i$.\\
$\{w^t_i\}_{i \in \arms} =$ \ConfidenceWidth($\delta$). (see description in text)\\
$C^t_{i_t}=$ \ChainedActions($\{w^t_i\}_{i \in \arms}$). (see description in text)\\
$j =$ Uniformly random selection from $C^t_{i_t}$.\\
$p^t_j = \theta_t.(\est^t_{i_t} - \est^t_j)$.\\
$p^t_j= \min(p^t_j,B)$ to ensure no budget overshooting. \\
Update budget $B=B-p^t_j$.\\
}
\textbf{return} $\mathbf{p^t}$.
}
\caption{\LimitedBudget}\label{alg:Limited_Budget}
\end{algorithm}
